# Supplementary material for: Stopping mass-selected alkaline-earth metal monofluoride beams of high energy via formation of unusually stable anions
Source: arXiv:2403.09320 source file (2024-05-14)
Supplement: Supplementary file 1 [file supplement.pdf]

# Supplementary Material for "Stopping mass-selected alkaline-earth metal monofluoride beams of high energy via formation of unusually stable anions"

Konstantin Gaul,<sup>1</sup> Ronald F. Garcia Ruiz,<sup>2</sup> and Robert Berger<sup>1</sup>

<sup>1</sup>*Fachbereich Chemie, Philipps-Universität Marburg, Hans-Meerwein-Straße 4, 35032 Marburg*

<sup>2</sup>*Massachusetts Institute of Technology, Cambridge, MA 02139, USA*

(Dated: March 14, 2024)

## I. COMPUTATIONAL DETAILS

Non-relativistic one-component coupled cluster calculations involving iterative singles and doubles amplitudes and perturbative triples amplitudes [CCSD(T)] were performed with the program package Molpro [1, 2]. Hereby, a large augmented quadruple zeta quality basis set, aug-cc-pVQZ, was used for Be, Mg and F. Large-core relativistic pseudopotentials, including all but 10 valence electrons, were used together with a aug-cc-pwCVQZ-PP basis set for Ca, Sr, Ba and Ra. In all CCSD(T) calculations only the lowest s-shell was frozen. For all-electron calculations of compounds involving Ca, the aug-cc-pVQZ basis set was employed for Ca.

With the very same basis sets an energy decomposition analysis (EDA) was performed on the Hartree–Fock (HF) level using symmetry adapted perturbation theory (SAPT) as implemented in Molpro [3]. Results are shown in Table II.

In order to account for relativistic effects in  $\text{RaF}^-$  beyond the pseudopotential approximation, the dissociation energy  $D_e$  and the ADE were computed at the relativistic four-component CCSD(T) [4c-CCSD(T)] level starting from the Dirac–Coulomb Hamiltonian using a Dyall basis set of quadruple-zeta quality (dyall.cv4z), [4, 5] and correlating the  $2s^22p^6$  shells of  $\text{F}^-$  and the  $5d^{10}6s^26p^27s^2$  shells of Ra explicitly in an active space with virtual spinors up to a cut-off energy of  $80 E_h$ . Excited electronic states were computed at the level of Equation-of-Motion 4c-CCSD (EOM-4c-CCSD) with the same active space and basis sets. Calculations of energies and oscillator strengths of the electronic transitions on the level of relativistic four-component time-dependent density functional theory (TDDFT) were performed with the CAMB3LYP exchange-correlation functional [6–9] and the dyall.cv3z basis set [4, 5]. To account for important contributions of very diffuse orbitals to the excitation energies, we repeated EOM-4c-CCSD and TDDFT-CAMB3LYP calculations with a doubly augmented dyall.cv4z basis set on Ra (EOM-4c-CCSDaug and TDDFT-CAMB3LYPaug). All four component relativistic calculations presented herein and in the main text were performed with the program package DIRAC19 [10].

In all four-component calculations a spherical Gaussian nuclear charge density distribution of form  $\rho_A(r) = \rho_0 \exp(-\zeta_A r^2)$  was assumed when calculating the electron-nuclear potential, where  $\zeta_A = 3/(2 \langle r^2 \rangle_A)$  and the root-mean-square nuclear radius  $\sqrt{\langle r^2 \rangle_A}$  was empirically determined as suggested in Ref. [11] using the isotopes  $^{226}\text{Ra}$  and  $^{19}\text{F}$ .

At the level of 4c-CCSD(T) we computed the Born–Oppenheimer potential energy curve and used a discrete variable representation (DVR) approach with an equally spaced grid to account for vibrational corrections (as detailed for instance in the appendix of Ref. [12]). Here, we used 1201 equidistant grid points in the range of  $1.9 \text{ \AA} \leq r_e \leq 3.01 \text{ \AA}$ . Harmonic vibrational wavenumbers were computed from a cubic fit of the 4c-CCSD(T) potential. DVR vibrational wave functions were employed to compute Franck–Condon factors.

From comparison of 4c-CCSD(T) to 4c-CCSD calculations in Table I and previous studies of  $\text{RaF}$  [13] we estimate the error of the dissociation energy and the ionization energy due to higher-order correlation effects to be  $< 1\%$  as

Table I. Dissociation wavenumber  $\tilde{D}_e$ , adiabatic photo-electron detachment wavenumber (ADW), equilibrium bond length  $r_e$ , harmonic vibrational wavenumber  $\tilde{\omega}_e$  of  $\text{RaF}^-$  and cumulative Franck–Condon factors  $f_v(N) = \sum_{i=0}^N \langle i | 0 \rangle$  for a transition of various vibrational levels of  $\text{RaF}^-$  from the vibrational ground state of  $\text{RaF}$  computed at the level of 4c-CCSD and 4c-CCSD(T) compared to RECP calculations. The number of digits of Franck–Condon factors does not reassemble its accuracy but merely is used to indicate the order of magnitude of the deviation from one.

| Method       | $\tilde{D}_e/\text{cm}^{-1}$ | ADW/ $\text{cm}^{-1}$ | $r_e/\text{\AA}$ | $\tilde{\omega}_e/\text{cm}^{-1}$ | $f_v(0)$ | $f_v(1)$ | $f_v(2)$ | $f_v(3)$ |
|--------------|------------------------------|-----------------------|------------------|-----------------------------------|----------|----------|----------|----------|
| RECP-HF      | 24 300                       | 1530                  | 2.34             | 375                               |          |          |          |          |
| RECP-CCSD(T) | 23 600                       | 7220                  | 2.36             | 401                               |          |          |          |          |
| 4c-HF        | 24 800                       | 1450                  | 2.32             | 378                               | 0.725    | 0.953    | 0.994    | 0.999    |
| 4c-CCSD      | 24 800                       | 7790                  | 2.31             | 382                               | 0.655    | 0.918    | 0.981    | 0.992    |
| 4c-CCSD(T)   | 25 000                       | 7060                  | 2.31             | 383                               | 0.648    | 0.922    | 0.987    | 0.998    |

Table II. Results of the SAPT and Mulliken partial charges  $\delta q$  of alkaline-earth metal monofluoride cations ( $\text{MF}^+$ ) and anions ( $\text{MF}^-$ ) at the level of all electron (AE) HF or RECP-HF (ECP). The contributions to the total bonding energy within SAPT are explained in the main text. The Mulliken partial charge of the metal atom is found by the difference of the total charge and  $\delta q_{\text{F}}$ . All energies are given in units of eV and the partial charge in units of  $e$ .

| Compound                  | $\Delta E_{\text{elstat}}$ | $\Delta E_{\text{ex}}$ | $\Delta E_{\text{ind,M} \rightarrow \text{F}}$ | $\Delta E_{\text{ind,F} \rightarrow \text{M}}$ | $\Delta E_{\text{dsp}}$ | $\Delta E_{\text{HF}}$ | $\Delta E_{\text{int}}$ | $\Delta E_{\text{prep}}$ | $\delta q_{\text{F}}$ |
|---------------------------|----------------------------|------------------------|------------------------------------------------|------------------------------------------------|-------------------------|------------------------|-------------------------|--------------------------|-----------------------|
| $\text{MF}^+$             |                            |                        |                                                |                                                |                         |                        |                         |                          |                       |
| $\text{BeF}^+/\text{AE}$  | -20.04                     | 3.96                   | -4.95                                          | -0.01                                          | -0.09                   | 0.02                   | -21.10                  | 0.02                     | -0.58                 |
| $\text{MgF}^+/\text{AE}$  | -17.15                     | 3.09                   | -2.56                                          | -0.02                                          | -0.11                   | 0.73                   | -16.01                  | 0.03                     | -0.72                 |
| $\text{CaF}^+/\text{AE}$  | -16.50                     | 5.11                   | -1.63                                          | -0.17                                          | -0.45                   | -0.40                  | -14.04                  | 0.11                     | -0.81                 |
| $\text{CaF}^+/\text{ECP}$ | -16.42                     | 5.58                   | -3.53                                          | -0.16                                          | -0.52                   | 0.94                   | -14.12                  | 0.18                     | -0.92                 |
| $\text{SrF}^+/\text{ECP}$ | -15.57                     | 5.33                   | -3.88                                          | -0.25                                          | -0.57                   | 1.69                   | -13.26                  | 0.16                     | -0.89                 |
| $\text{BaF}^+/\text{ECP}$ | -15.16                     | 5.77                   | -4.55                                          | -0.39                                          | -0.69                   | 2.32                   | -12.70                  | 0.18                     | -0.83                 |
| $\text{RaF}^+/\text{ECP}$ | -14.57                     | 5.15                   | -4.02                                          | -0.43                                          | -0.66                   | 2.25                   | -12.28                  | 0.17                     | -0.83                 |
| $\text{MF}^-$             |                            |                        |                                                |                                                |                         |                        |                         |                          |                       |
| $\text{BeF}^-/\text{AE}$  | -7.39                      | 8.60                   | -1.51                                          | -0.17                                          | -1.58                   | -2.42                  | -4.47                   | 0.65                     | -0.79                 |
| $\text{MgF}^-/\text{AE}$  | -4.77                      | 4.80                   | -0.62                                          | -0.94                                          | -1.04                   | -0.68                  | -3.23                   | 0.53                     | -0.81                 |
| $\text{CaF}^-/\text{AE}$  | -5.22                      | 4.95                   | -0.54                                          | -1.00                                          | -1.05                   | -0.96                  | -3.81                   | 0.54                     | -0.97                 |
| $\text{CaF}^-/\text{ECP}$ | -5.15                      | 5.09                   | -1.81                                          | -0.97                                          | -1.11                   | 0.11                   | -3.83                   | 0.55                     | -0.96                 |
| $\text{SrF}^-/\text{ECP}$ | -4.82                      | 4.68                   | -2.08                                          | -1.09                                          | -1.05                   | 0.64                   | -3.72                   | 0.53                     | -0.94                 |
| $\text{BaF}^-/\text{ECP}$ | -4.96                      | 4.81                   | -2.58                                          | -1.16                                          | -1.04                   | 1.03                   | -3.91                   | 0.50                     | -0.88                 |
| $\text{RaF}^-/\text{ECP}$ | -4.48                      | 4.36                   | -2.22                                          | -1.22                                          | -1.00                   | 1.07                   | -3.49                   | 0.48                     | -0.89                 |

only closed shell species are involved, whereas for the ADE we estimate this error to be  $< 5\%$  as open-shell  $\text{RaF}$  is involved. The effect of a larger basis sets and a larger active space is estimated to be below 4%.

Following the same arguments we can estimate the relative error of excitation energies from EOM-4c-CCSD calculations to be less than 20%. This uncertainty estimate includes accounting for effects of very diffuse orbitals that can lower the excitation energies, which were estimated for vertical excitation energies by doubly augmenting the basis set. Thereby, we note that this basis set augmentation lowers vertical excitation wavenumbers in  $\text{RaF}^-$  by about  $400 \text{ cm}^{-1}$  (see Tab. III).

Table III. Spectroscopic properties of electronically excited states of  $\text{RaF}^-$  computed at the level of EOM-4c-CCSD within the adiabatic approximation (adb) and vertical approximation (vrt) at the equilibrium bond length of the ground state as well as at the level of TDDFT-CAMB3LYP in the vertical approximation. Calculations in the vertical approximation were performed at a bond length of 2.3 Å. Equilibrium bond-length  $r_e$ , harmonic vibrational wavenumbers  $\tilde{\omega}_e$  and cumulated Franck–Condon factors  $f_v(N) = \sum_{i=0}^N \langle i | 0 \rangle$  for relevant transitions from vibrational excited states in the electronic ground states to the vibrational ground state of the electronically excited state are computed at the level of EOM-4c-CCSD. Electronic oscillator strength  $f_e$  is given at the level of TDDFT-CAMB3LYP.

| State             | Method                        | $\tilde{T}_e/\text{cm}^{-1}$ | $10^3 f_e$ | $r_e/\text{\AA}$ | $\tilde{\omega}_e/\text{cm}^{-1}$ | $f_v(0)$ | $f_v(1)$ | $f_v(2)$ |
|-------------------|-------------------------------|------------------------------|------------|------------------|-----------------------------------|----------|----------|----------|
| (1)0 <sup>-</sup> | EOM-4c-CCSD(adb)              | 6660                         |            | 2.28             | 402                               |          |          |          |
|                   | EOM-4c-CCSD(vrt)              | 6680                         |            |                  |                                   |          |          |          |
|                   | EOM-4c-CCSDaug(vrt)           | 6250                         |            |                  |                                   |          |          |          |
|                   | TDDFT-CAMB3LYP                | 6100                         | 0          |                  |                                   |          |          |          |
|                   | TDDFT-CAMB3LYP <sub>aug</sub> | 5230                         | 0          |                  |                                   |          |          |          |
| (2)0 <sup>+</sup> | EOM-4c-CCSD(adb)              | 6740                         |            | 2.28             | 403                               | 0.912 30 | 0.994 66 | 0.999 71 |
|                   | EOM-4c-CCSD(vrt)              | 6760                         |            |                  |                                   |          |          |          |
|                   | EOM-4c-CCSDaug(vrt)           | 6340                         |            |                  |                                   |          |          |          |
|                   | TDDFT-CAMB3LYP                | 6210                         | 0.379      |                  |                                   |          |          |          |
|                   | TDDFT-CAMB3LYP <sub>aug</sub> | 5340                         | 0.387      |                  |                                   |          |          |          |
| (1)1              | EOM-4c-CCSD(adb)              | 7160                         |            | 2.28             | 405                               | 0.896 77 | 0.992 71 | 0.999 55 |
|                   | EOM-4c-CCSD(vrt)              | 7190                         |            |                  |                                   |          |          |          |
|                   | EOM-4c-CCSDaug(vrt)           | 6700                         |            |                  |                                   |          |          |          |
|                   | TDDFT-CAMB3LYP                | 6750                         | 1.38       |                  |                                   |          |          |          |
|                   | TDDFT-CAMB3LYP <sub>aug</sub> | 5710                         | 0.800      |                  |                                   |          |          |          |
| (1)2              | EOM-4c-CCSD(vrt)              | 7730                         |            |                  |                                   |          |          |          |
|                   | EOM-4c-CCSDaug(vrt)           | 7150                         |            |                  |                                   |          |          |          |
|                   | TDDFT-CAMB3LYP                | 7430                         | 0          |                  |                                   |          |          |          |
|                   | TDDFT-CAMB3LYP <sub>aug</sub> | 6050                         | 0          |                  |                                   |          |          |          |

- 
- [1] H.-J. Werner, P. J. Knowles, G. Knizia, F. R. Manby, M. Schütz, P. Celani, W. Györffy, D. Kats, T. Korona, R. Lindh, A. Mitrushenkov, G. Rauhut, K. R. Shamasundar, T. B. Adler, R. D. Amos, S. J. Bennie, A. Bernhardsson, A. Berning, D. L. Cooper, M. J. O. Deegan, A. J. Dobbyn, F. Eckert, E. Goll, C. Hampel, A. Hesselmann, G. Hetzer, T. Hrenar, G. Jansen, C. Köppl, S. J. R. Lee, Y. Liu, A. W. Lloyd, Q. Ma, R. A. Mata, A. J. May, S. J. McNicholas, W. Meyer, T. F. Miller III, M. E. Mura, A. Nicklass, D. P. O'Neill, P. Palmieri, D. Peng, K. Pflüger, R. Pitzer, M. Reiher, T. Shiozaki, H. Stoll, A. J. Stone, R. Tarroni, T. Thorsteinsson, M. Wang, and M. Welborn, “Molpro, version 2019.2, a package of ab initio programs,” (2019), see <http://www.molpro.net>.
- [2] H.-J. Werner, P. J. Knowles, F. R. Manby, J. A. Black, K. Doll, A. Heßelmann, D. Kats, A. Köhn, T. Korona, D. A. Kreplin, Q. Ma, T. F. Miller, A. Mitrushchenkov, K. A. Peterson, I. Polyak, G. Rauhut, and M. Sibaev, *J. Chem. Phys.* **152**, 144107 (2020), <https://doi.org/10.1063/5.0005081>.
- [3] B. Jeziorski, R. Moszynski, and K. Szalewicz, *Chem. Rev.* **94**, 1887 (1994), <https://doi.org/10.1021/cr00031a008>.
- [4] K. G. Dyall, *Theor. Chem. Acc.* **108**, 335 (2002).
- [5] K. G. Dyall, *Theor. Chem. Acc.* **115**, 441 (2006).
- [6] S. H. Vosko, L. Wilk, and M. Nuisar, *Can. J. Phys.* **58**, 1200 (1980).
- [7] P. J. Stephens, F. J. Devlin, C. F. Chabalowski, and M. J. Frisch, *J. Phys. Chem.* **98**, 11623 (1994).
- [8] A. D. Becke, *Phys. Rev. A* **38**, 3098 (1988).
- [9] T. Yanai, D. P. Tew, and N. C. Handy, *Chem. Phys. Lett.* **393**, 51 (2004).
- [10] DIRAC, a relativistic ab initio electronic structure program, Release DIRAC19 (2019), written by A. S. P. Gomes, T. Saue, L. Visscher, H. J. Aa. Jensen, and R. Bast, with contributions from I. A. Aucar, V. Bakken, K. G. Dyall, S. Dubillard, U. Ekström, E. Eliav, T. Enevoldsen, E. Faßhauer, T. Fleig, O. Fossgaard, L. Halbert, E. D. Hedegård, B. Heimlich–Paris, T. Helgaker, J. Henriksson, M. Iliaš, Ch. R. Jacob, S. Knecht, S. Komorovský, O. Kullie, J. K. Lærdahl, C. V. Larsen, Y. S. Lee, H. S. Nataraj, M. K. Nayak, P. Norman, G. Olejniczak, J. Olsen, J. M. H. Olsen, Y. C. Park, J. K. Pedersen, M. Pernpointner, R. di Remigio, K. Ruud, P. Salek, B. Schimmelpfennig, B. Senjean, A. Shee, J. Sikkema, A. J. Thorvaldsen, J. Thyssen, J. van Stralen, M. L. Vidal, S. Villaume, O. Visser, T. Winther, and S. Yamamoto (available at <http://dx.doi.org/10.5281/zenodo.3572669>, see also <http://www.diracprogram.org>).
- [11] L. Visscher and K. G. Dyall, *At. Data Nucl. Data Tables* **67**, 207 (1997).
- [12] S. M. Udrescu, A. J. Brinson, R. F. G. Ruiz, K. Gaul, R. Berger, J. Billowes, C. L. Binnersley, M. L. Bissell, A. A. Breier, K. Chrysalidis, T. E. Cocolios, B. S. Cooper, K. T. Flanagan, T. F. Giesen, R. P. de Groote, S. Franchoo, F. P. Gustafsson, T. A. Isaev, A. Koszorus, G. Neyens, H. A. Perrett, C. M. Ricketts, S. Rothe, A. R. Vernon, K. D. A. Wendt, F. Wienholtz, S. G. Wilkins, and X. F. Yang, *Phys. Rev. Lett.* **127**, 033001 (2021), [arXiv:2105.10549 \[nucl-ex\]](https://arxiv.org/abs/2105.10549).
- [13] A. Zaitsevskii, L. V. Skripnikov, N. S. Mosyagin, T. Isaev, R. Berger, A. A. Breier, and T. Giesen, *J. Chem. Phys.* **in press** (2022), 10.1063/5.0079618, <https://doi.org/10.1063/5.0079618>.
